# Supplementary material for: HADAD: A Lightweight Approach for Optimizing Hybrid Complex Analytics Queries (Extended Version)
Source: arXiv:2103.12317 source file (2021-03-23)
Supplement: Supplementary file 1 [file appendixH.tex]

\onecolumn
\section{Hybrid Twitter Benchmark Constraints }
\counterwithin{lstlisting}{section}
\eat{\RA{Simplified version}}
\lstdefinestyle{myCustomMatlabStyle}{
  numbers=left,
  stepnumber=1,
  numbersep=10pt,
  tabsize=4,
  showspaces=false,
  showstringspaces=false
}
\lstset{basicstyle=\tiny,style=myCustomMatlabStyle}
\begin{lstlisting}[caption={Forward Constraints Used for Q1 },captionpos=b]
#EGDs
$name(id1,n1),name(id2,n1)->id2=id1;$
$tr(id1,idt1),tr(id1,idt2)->idt2=idt1;$
$in(id1,idt1),in(id1,idt2)->idt2=idt1;$
$ins(id1,idt1),ins(id1,idt2)->idt1=idt2;$
$in(id1,idr1),in(idr1,idr3)->idr3=id1;$
$multi(idA,idB,idr1),multi(idA,idB,idr2)->idr2=idr1;$
$multi_s(idA,idB,idr1),multi_s(idA,idB,idr2)->idr2=idr1;$
$det(idA,d1),det(idA,d2)->d2=d1;$
$trace(idA,id1),trace(idA,id2)->id2=id1;$
$add(idA,idB,idr1),add(idA,idB,idr2)->idr1=idr2;$
$size(idA,i1,j1),size(idA,i2,j2)->j2=j1,i2=i1;$
$name(id1,n1),name(id2,n1)->id2=id1;$
$nameI(mID1,n1),nameI(mID1,n2)->n1=n2;$
$add_s(idA,idB,idr1),add_s(idA,idB,idr2)->idr1=idr2;$
$sum(id1,idt1),sum(id1,idt2)->idt2=idt1;$
$rowSums(idA,id1),rowSums(idA,id2)->id2=id1;$
$colSums(idA,id1),colSums(idA,id2)->id2=id1;$
$user(EID, FOLC1,FRIC1,LC1,P1,V1),user(EID, FOLC2,FRIC2,LC2,P2,V2)-> FOLC2=FOLC1,FRIC2=FRIC1,LC2=LC1,P2=P1,V2=V1;$
$constructMatrix_2(rID,mID,v11,v12),constructMatrix_2(rID,mID,v21,v22)-> v21=v11,v22=v12;$
$constructMatrix_4(rID,mID,v11,v12,v13,v14),constructMatrix_4(rID,mID,v21,v22,v23,v24)->v21=v11,v22=v12,v23=v13,v24=v14;$
$constructMatrix_{11}(rID,mID,v11,v12,v13,v14,v15,v16,v17,v18,v19,v110,v111), constructMatrix_{11}(rID,mID,v21,v22,v23,v24,v25,v26,v27,v28,v29,v210,v211)->$
$v11=v21,v12=v22,v13=vv23,v14=v24,v15=v25,v16=v26,v17=v27,v18=v28,v19=v29,v110=v210,v111=v211;$
$constructMtxMatrix(i,j,v,id)(i1,j1,v1,id),constructMtxMatrix(i2,j2,v2,id)-> i2=i1,j2=j1,v2=v1;$
$indicator(id1,id2,idr31),indicator(id1,id2,idr32)->idr32=idr31;$
$deriveFrom(id1,id2,idr31),deriveFrom(id1,id2,idr32)-> idr32=idr31;$
$concat(id1,id2,idr1),concat(id1,id2,idr2)->idr2=idr1;$
$subset_{tweet}(id1,id2,id3,id4,id5,id6,id7,idr1),$
$subset_{tweet}(id1,id2,id3,id4,id5,id6,id7,idr2)->idr2=idr1;$
$subset_{user}(id1,id2,id3,id4,id5,id6,idr1),$
$subset_{user}(id1,id2,id3,id4,id5,id6,idr2)->idr2=idr1;$
$tweet(id1),tweet(id2)->id2=id1;$
$child_{sp}(x,y1,z,d),child_{sp}(x,y2,z,d)->y2=y1;$
$val_{sp}(x,v1),val_{sp}(x,v2)->v2=v1;$
$child_{{sj}_{V2}}(x,y1,z,d),child_{{sj}_{V2}}(x,y2,z,d)->y2=y1;$

#TGDs
$add(idA,idB,idr1)->add(idB,idA,idr1);$
$multi(id1,id2,idr1),rowSums(idr1,idr2)->rowSums(id2,idr3),multi(id1,idr3,idr2);$
$add(idA,idB,idr1),multi(idr1,idC,idr2)->multi(idA,idC,c1),multi(idB,idC,c2),add(c1,c2,idr2);$
$multi(idA,idB,idr1),multi(idr1,idC,idr2)-> multi(idB,idC,idr3),multi(idA,idr3,idr2);$
$add(idA,idB,idr1),tr(idr1,idT)->tr(idA,idAT),tr(idB,idBT),add(idAT,idBT,idT);$
$tr(idA,idAT),tr(idB,idBT),multi(idBT,idAT,idr2)->multi(idA,idB,idr1),tr(idr1,idr2);$
$construcMtxMatrix(i,j,v,id),name(id,n),matrixFilterLT(id,x,idr1)->$
$name(idr1,n),construcMtxMatrix(i,j,v,idr1),LT(v,x);$

$subset_{tweet}(mID2,"FC", "QC","RC","F","PS","R",idS1),$
$subset_{user}(mID3,"FOLC","FRIC","LC","P","V",idR1),$
$indicator(mID2,mID3,idK),deriveFrom(idS1,idR1,id),rowSums(id,idr1)->$
$rowSums(idS1,idr2),rowSums(idR1,idr3),multi(idK,idr3,idr4),add(idr2,idr4,idr1);$

$user(EID,FOLC,FRIC,LC,P,V),$
$tweetR(EID,FC, QC,RC,F,PS,R),$
$constructMatrix_{11}(mID1,rwID,FOLC,FRIC,LC,P,V,FC,QC,RC,F,PS,R)->$
$nameI(mID1,n),$
$name(mID2,"tweet"),$
$name(mID3,"user"),$
$subset_{tweet}(mID2,"FC", "QC","RC","F","PS","R",idS1),$
$subset_{user}(mID3,"FOLC","FRIC","LC","P","V",idR1),$
$indicator(mID2,mID3,idr3),$
$deriveFrom(idS1,idR1,mID1);$
$name(idS,"tweet"),$
$name(idR,"user"),$
$indicator(idS,idR,idK),$
$subset_{tweet}(idS,"FC", "QC","RC","F","PS","R",idS1),$
$subset_{user}(idR,"FOLC","FRIC","LC","P","V",idR1),$
$rowSums(idS1,idr1),$
$rowSums(idR1,idr2),$
$multi(idK,idr2,idr3),$
$add(idr1,idr3,idr4)->name(idr4,"VV1");$

$tweet(id),$
$child_{sp}(id,"tweetID","o",tID),$
$child_{sp}(id,"flevel","o",fID),$
$child_{sp}(id,"entities","o",eID),$
$child_{sp}(eID,"hashtag","o",hID),$
$child_{sp}(hID,"hID","o",hcID),$
$child_{sp}(id,"place","o",pID),$
$child_{sp}(pID,"code","o",cID)->V1(tID,hcID,fID,cID);$

$tweet(id),$
$child_{sp}(id,"tweetID","o",tID),$
$child_{sp}(id,"text","o",text)->$
$V2(idV2),$
$child_{{sj}_{V2}}(idV2,"tweetID","o",tID),$
$child_{{sj}_{V2}}(idV2,"text","o",text);$
\end{lstlisting}

\newpage
\begin{lstlisting}[caption={Forward Constraints Used for Q2 },captionpos=b]
#EGDs
$name(id1,n1),name(id2,n1)->id2=id1;$
$tr(id1,idt1),tr(id1,idt2)->idt2=idt1;$
$in(id1,idt1),in(id1,idt2)->idt2=idt1;$
$ins(id1,idt1),ins(id1,idt2)->idt1=idt2;$
$in(id1,idr1),in(idr1,idr3)->idr3=id1;$
$multi(idA,idB,idr1),multi(idA,idB,idr2)->idr2=idr1;$
$multi_s(idA,idB,idr1),multi_s(idA,idB,idr2)->idr2=idr1;$
$det(idA,d1),det(idA,d2)->d2=d1;$
$trace(idA,id1),trace(idA,id2)->id2=id1;$
$add(idA,idB,idr1),add(idA,idB,idr2)->idr1=idr2;$
$size(idA,i1,j1),size(idA,i2,j2)->j2=j1,i2=i1;$
$name(id1,n1),name(id2,n1)->id2=id1;$
$nameI(mID1,n1),nameI(mID1,n2)->n1=n2;$
$add_s(idA,idB,idr1),add_s(idA,idB,idr2)->idr1=idr2;$
$sum(id1,idt1),sum(id1,idt2)->idt2=idt1;$
$rowSums(idA,id1),rowSums(idA,id2)->id2=id1;$
$colSums(idA,id1),colSums(idA,id2)->id2=id1;$
$user(EID, FOLC1,FRIC1,LC1,P1,V1),user(EID, FOLC2,FRIC2,LC2,P2,V2)-> FOLC2=FOLC1,FRIC2=FRIC1,LC2=LC1,P2=P1,V2=V1;$
$constructMatrix_2(rID,mID,v11,v12),constructMatrix_2(rID,mID,v21,v22)-> v21=v11,v22=v12;$
$constructMatrix_4(rID,mID,v11,v12,v13,v14),constructMatrix_4(rID,mID,v21,v22,v23,v24)->v21=v11,v22=v12,v23=v13,v24=v14;$
$constructMatrix_{11}(rID,mID,v11,v12,v13,v14,v15,v16,v17,v18,v19,v110,v111), constructMatrix_{11}(rID,mID,v21,v22,v23,v24,v25,v26,v27,v28,v29,v210,v211)->$
$v11=v21,v12=v22,v13=vv23,v14=v24,v15=v25,v16=v26,v17=v27,v18=v28,v19=v29,v110=v210,v111=v211;$
$constructMtxMatrix(i,j,v,id)(i1,j1,v1,id),constructMtxMatrix(i2,j2,v2,id)-> i2=i1,j2=j1,v2=v1;$
$indicator(id1,id2,idr31),indicator(id1,id2,idr32)->idr32=idr31;$
$deriveFrom(id1,id2,idr31),deriveFrom(id1,id2,idr32)-> idr32=idr31;$
$concat(id1,id2,idr1),concat(id1,id2,idr2)->idr2=idr1;$
$subset_{tweet}(id1,id2,id3,id4,id5,id6,id7,idr1),$
$subset_{tweet}(id1,id2,id3,id4,id5,id6,id7,idr2)->idr2=idr1;$
$subset_{user}(id1,id2,id3,id4,id5,id6,idr1),$
$subset_{user}(id1,id2,id3,id4,id5,id6,idr2)->idr2=idr1;$
$tweet(id1),tweet(id2)->id2=id1;$
$child_{sp}(x,y1,z,d),child_{sp}(x,y2,z,d)->y2=y1;$
$val_{sp}(x,v1),val_{sp}(x,v2)->v2=v1;$
$child_{{sj}_{V2}}(x,y1,z,d),child_{{sj}_{V2}}(x,y2,z,d)->y2=y1;$

#TGDs
$add(idA,idB,idr1)->add(idB,idA,idr1);$
$multi(id1,id2,idr1),rowSums(idr1,idr2)->rowSums(id2,idr3),multi(id1,idr3,idr2);$
$add(idA,idB,idr1),multi(idr1,idC,idr2)->multi(idA,idC,c1),multi(idB,idC,c2),add(c1,c2,idr2);$
$multi(idA,idB,idr1),multi(idr1,idC,idr2)-> multi(idB,idC,idr3),multi(idA,idr3,idr2);$
$add(idA,idB,idr1),tr(idr1,idT)->tr(idA,idAT),tr(idB,idBT),add(idAT,idBT,idT);$
$tr(idA,idAT),tr(idB,idBT),multi(idBT,idAT,idr2)->multi(idA,idB,idr1),tr(idr1,idr2);$
$construcMtxMatrix(i,j,v,id),name(id,n),matrixFilterLT(id,x,idr1)->$
$name(idr1,n),construcMtxMatrix(i,j,v,idr1),LT(v,x);$
$tr(id,idr1),colSums(idr1,idr2)->rowSums(id,idr3),tr(idr3,idr2);$

$subset_{tweet}(mID2,"FC", "QC","RC","F","PS","R",idS1),$
$subset_{user}(mID3,"FOLC","FRIC","LC","P","V",idR1),$
$indicator(mID2,mID3,idK),deriveFrom(idS1,idR1,id),rowSums(id,idr1)->$
$rowSums(idS1,idr2),rowSums(idR1,idr3),multi(idK,idr3,idr4),add(idr2,idr4,idr1);$

$user(EID,FOLC,FRIC,LC,P,V),$
$tweetR(EID,FC, QC,RC,F,PS,R),$
$constructMatrix_{11}(mID1,rwID,FOLC,FRIC,LC,P,V,FC,QC,RC,F,PS,R)->$
$nameI(mID1,n),$
$name(mID2,"tweet"),$
$name(mID3,"user"),$
$subset_{tweet}(mID2,"FC", "QC","RC","F","PS","R",idS1),$
$subset_{user}(mID3,"FOLC","FRIC","LC","P","V",idR1),$
$indicator(mID2,mID3,idr3),$
$deriveFrom(idS1,idR1,mID1);$
$name(idS,"tweet"),$
$name(idR,"user"),$
$indicator(idS,idR,idK),$
$subset_{tweet}(idS,"FC", "QC","RC","F","PS","R",idS1),$
$subset_{user}(idR,"FOLC","FRIC","LC","P","V",idR1),$
$rowSums(idS1,idr1),$
$rowSums(idR1,idr2),$
$multi(idK,idr2,idr3),$
$add(idr1,idr3,idr4)->name(idr4,"VV1");$

$tweet(id),$
$child_{sp}(id,"tweetID","o",tID),$
$child_{sp}(id,"flevel","o",fID),$
$child_{sp}(id,"entities","o",eID),$
$child_{sp}(eID,"hashtag","o",hID),$
$child_{sp}(hID,"hID","o",hcID),$
$child_{sp}(id,"place","o",pID),$
$child_{sp}(pID,"code","o",cID)->V1(tID,hcID,fID,cID);$

$tweet(id),$
$child_{sp}(id,"tweetID","o",tID),$
$child_{sp}(id,"text","o",text)->$
$V2(idV2),$
$child_{{sj}_{V2}}(idV2,"tweetID","o",tID),$
$child_{{sj}_{V2}}(idV2,"text","o",text);$
\end{lstlisting}

\newpage
\begin{lstlisting}[caption={Forward Constraints Used for Q3 },captionpos=b]
#EGDs
$name(id1,n1),name(id2,n1)->id2=id1;$
$tr(id1,idt1),tr(id1,idt2)->idt2=idt1;$
$in(id1,idt1),in(id1,idt2)->idt2=idt1;$
$ins(id1,idt1),ins(id1,idt2)->idt1=idt2;$
$in(id1,idr1),in(idr1,idr3)->idr3=id1;$
$multi(idA,idB,idr1),multi(idA,idB,idr2)->idr2=idr1;$
$multi_s(idA,idB,idr1),multi_s(idA,idB,idr2)->idr2=idr1;$
$det(idA,d1),det(idA,d2)->d2=d1;$
$trace(idA,id1),trace(idA,id2)->id2=id1;$
$add(idA,idB,idr1),add(idA,idB,idr2)->idr1=idr2;$
$size(idA,i1,j1),size(idA,i2,j2)->j2=j1,i2=i1;$
$name(id1,n1),name(id2,n1)->id2=id1;$
$nameI(mID1,n1),nameI(mID1,n2)->n1=n2;$
$add_s(idA,idB,idr1),add_s(idA,idB,idr2)->idr1=idr2;$
$sum(id1,idt1),sum(id1,idt2)->idt2=idt1;$
$rowSums(idA,id1),rowSums(idA,id2)->id2=id1;$
$colSums(idA,id1),colSums(idA,id2)->id2=id1;$
$user(EID, FOLC1,FRIC1,LC1,P1,V1),user(EID, FOLC2,FRIC2,LC2,P2,V2)-> FOLC2=FOLC1,FRIC2=FRIC1,LC2=LC1,P2=P1,V2=V1;$
$constructMatrix_2(rID,mID,v11,v12),constructMatrix_2(rID,mID,v21,v22)-> v21=v11,v22=v12;$
$constructMatrix_4(rID,mID,v11,v12,v13,v14),constructMatrix_4(rID,mID,v21,v22,v23,v24)->v21=v11,v22=v12,v23=v13,v24=v14;$
$constructMatrix_{11}(rID,mID,v11,v12,v13,v14,v15,v16,v17,v18,v19,v110,v111), constructMatrix_{11}(rID,mID,v21,v22,v23,v24,v25,v26,v27,v28,v29,v210,v211)->$
$v11=v21,v12=v22,v13=vv23,v14=v24,v15=v25,v16=v26,v17=v27,v18=v28,v19=v29,v110=v210,v111=v211;$
$constructMtxMatrix(i,j,v,id)(i1,j1,v1,id),constructMtxMatrix(i2,j2,v2,id)-> i2=i1,j2=j1,v2=v1;$
$indicator(id1,id2,idr31),indicator(id1,id2,idr32)->idr32=idr31;$
$deriveFrom(id1,id2,idr31),deriveFrom(id1,id2,idr32)-> idr32=idr31;$
$concat(id1,id2,idr1),concat(id1,id2,idr2)->idr2=idr1;$
$subset_{tweet}(id1,id2,id3,id4,id5,id6,id7,idr1),$
$subset_{tweet}(id1,id2,id3,id4,id5,id6,id7,idr2)->idr2=idr1;$
$subset_{user}(id1,id2,id3,id4,id5,id6,idr1),$
$subset_{user}(id1,id2,id3,id4,id5,id6,idr2)->idr2=idr1;$
$tweet(id1),tweet(id2)->id2=id1;$
$child_{sp}(x,y1,z,d),child_{sp}(x,y2,z,d)->y2=y1;$
$val_{sp}(x,v1),val_{sp}(x,v2)->v2=v1;$
$child_{{sj}_{V2}}(x,y1,z,d),child_{{sj}_{V2}}(x,y2,z,d)->y2=y1;$

#TGDs
$add(idA,idB,idr1)->add(idB,idA,idr1);$
$multi(id1,id2,idr1),rowSums(idr1,idr2)->rowSums(id2,idr3),multi(id1,idr3,idr2);$
$add(idA,idB,idr1),multi(idr1,idC,idr2)->multi(idA,idC,c1),multi(idB,idC,c2),add(c1,c2,idr2);$
$multi(idA,idB,idr1),multi(idr1,idC,idr2)-> multi(idB,idC,idr3),multi(idA,idr3,idr2);$
$construcMtxMatrix(i,j,v,id),name(id,n),matrixFilterLT(id,x,idr1)->$
$name(idr1,n),construcMtxMatrix(i,j,v,idr1),LT(v,x);$
$add(idA,idB,idr1),multi(idr1,idC,idr2)->multi(idA,idC,c1),multi(idB,idC,c2),add(c1,c2,idr2);$

$subset_{tweet}(mID2,"FC", "QC","RC","F","PS","R",idS1),$
$subset_{user}(mID3,"FOLC","FRIC","LC","P","V",idR1),$
$indicator(mID2,mID3,idK),deriveFrom(idS1,idR1,id),colSums(id,idr1)->$
$colSums(idK,idr2),multi(idr2,idR1,idr3),colSums(idS1,idr4),concat(idr4,idr3,idr1);$


$user(EID,FOLC,FRIC,LC,P,V),$
$tweetR(EID,FC, QC,RC,F,PS,R),$
$constructMatrix_{11}(mID1,rwID,FOLC,FRIC,LC,P,V,FC,QC,RC,F,PS,R)->$
$nameI(mID1,n),$
$name(mID2,"tweet"),$
$name(mID3,"user"),$
$subset_{tweet}(mID2,"FC", "QC","RC","F","PS","R",idS1),$
$subset_{user}(mID3,"FOLC","FRIC","LC","P","V",idR1),$
$indicator(mID2,mID3,idr3),$
$deriveFrom(idS1,idR1,mID1);$
$name(idS,"tweet"),$
$name(idR,"user"),$
$indicator(idS,idR,idK),$
$subset_{tweet}(idS,"FC", "QC","RC","F","PS","R",idS1),$
$subset_{user}(idR,"FOLC","FRIC","LC","P","V",idR1),$
$rowSums(idS1,idr1),$
$rowSums(idR1,idr2),$
$multi(idK,idr2,idr3),$
$add(idr1,idr3,idr4)->name(idr4,"VV1");$

$tweet(id),$
$child_{sp}(id,"tweetID","o",tID),$
$child_{sp}(id,"flevel","o",fID),$
$child_{sp}(id,"entities","o",eID),$
$child_{sp}(eID,"hashtag","o",hID),$
$child_{sp}(hID,"hID","o",hcID),$
$child_{sp}(id,"place","o",pID),$
$child_{sp}(pID,"code","o",cID)->V1(tID,hcID,fID,cID);$

$tweet(id),$
$child_{sp}(id,"tweetID","o",tID),$
$child_{sp}(id,"text","o",text)->$
$V2(idV2),$
$child_{{sj}_{V2}}(idV2,"tweetID","o",tID),$
$child_{{sj}_{V2}}(idV2,"text","o",text);$
\end{lstlisting}

\newpage
\begin{lstlisting}[caption={Forward Constraints Used for Q4 },captionpos=b]
#EGDs
$name(id1,n1),name(id2,n1)->id2=id1;$
$tr(id1,idt1),tr(id1,idt2)->idt2=idt1;$
$in(id1,idt1),in(id1,idt2)->idt2=idt1;$
$ins(id1,idt1),ins(id1,idt2)->idt1=idt2;$
$in(id1,idr1),in(idr1,idr3)->idr3=id1;$
$multi(idA,idB,idr1),multi(idA,idB,idr2)->idr2=idr1;$
$multi_s(idA,idB,idr1),multi_s(idA,idB,idr2)->idr2=idr1;$
$det(idA,d1),det(idA,d2)->d2=d1;$
$trace(idA,id1),trace(idA,id2)->id2=id1;$
$add(idA,idB,idr1),add(idA,idB,idr2)->idr1=idr2;$
$size(idA,i1,j1),size(idA,i2,j2)->j2=j1,i2=i1;$
$name(id1,n1),name(id2,n1)->id2=id1;$
$nameI(mID1,n1),nameI(mID1,n2)->n1=n2;$
$add_s(idA,idB,idr1),add_s(idA,idB,idr2)->idr1=idr2;$
$sum(id1,idt1),sum(id1,idt2)->idt2=idt1;$
$rowSums(idA,id1),rowSums(idA,id2)->id2=id1;$
$colSums(idA,id1),colSums(idA,id2)->id2=id1;$
$user(EID, FOLC1,FRIC1,LC1,P1,V1),user(EID, FOLC2,FRIC2,LC2,P2,V2)-> FOLC2=FOLC1,FRIC2=FRIC1,LC2=LC1,P2=P1,V2=V1;$
$constructMatrix_2(rID,mID,v11,v12),constructMatrix_2(rID,mID,v21,v22)-> v21=v11,v22=v12;$
$constructMatrix_4(rID,mID,v11,v12,v13,v14),constructMatrix_4(rID,mID,v21,v22,v23,v24)->v21=v11,v22=v12,v23=v13,v24=v14;$
$constructMatrix_{11}(rID,mID,v11,v12,v13,v14,v15,v16,v17,v18,v19,v110,v111), constructMatrix_{11}(rID,mID,v21,v22,v23,v24,v25,v26,v27,v28,v29,v210,v211)->$
$v11=v21,v12=v22,v13=vv23,v14=v24,v15=v25,v16=v26,v17=v27,v18=v28,v19=v29,v110=v210,v111=v211;$
$constructMtxMatrix(i,j,v,id)(i1,j1,v1,id),constructMtxMatrix(i2,j2,v2,id)-> i2=i1,j2=j1,v2=v1;$
$indicator(id1,id2,idr31),indicator(id1,id2,idr32)->idr32=idr31;$
$deriveFrom(id1,id2,idr31),deriveFrom(id1,id2,idr32)-> idr32=idr31;$
$concat(id1,id2,idr1),concat(id1,id2,idr2)->idr2=idr1;$
$subset_{tweet}(id1,id2,id3,id4,id5,id6,id7,idr1),$
$subset_{tweet}(id1,id2,id3,id4,id5,id6,id7,idr2)->idr2=idr1;$
$subset_{user}(id1,id2,id3,id4,id5,id6,idr1),$
$subset_{user}(id1,id2,id3,id4,id5,id6,idr2)->idr2=idr1;$
$tweet(id1),tweet(id2)->id2=id1;$
$child_{sp}(x,y1,z,d),child_{sp}(x,y2,z,d)->y2=y1;$
$val_{sp}(x,v1),val_{sp}(x,v2)->v2=v1;$
$child_{{sj}_{V2}}(x,y1,z,d),child_{{sj}_{V2}}(x,y2,z,d)->y2=y1;$

#TGDs
$add(idA,idB,idr1)->add(idB,idA,idr1);$
$multi(id1,id2,idr1),rowSums(idr1,idr2)->rowSums(id2,idr3),multi(id1,idr3,idr2);$
$add(idA,idB,idr1),multi(idr1,idC,idr2)->multi(idA,idC,c1),multi(idB,idC,c2),add(c1,c2,idr2);$
$multi(idA,idB,idr1),multi(idr1,idC,idr2)-> multi(idB,idC,idr3),multi(idA,idr3,idr2);$
$construcMtxMatrix(i,j,v,id),name(id,n),matrixFilterLT(id,x,idr1)->$
$name(idr1,n),construcMtxMatrix(i,j,v,idr1),LT(v,x);$
$add(idA,idB,idr1),multi(idr1,idC,idr2)->multi(idA,idC,c1),multi(idB,idC,c2),add(c1,c2,idr2);$


$subset_{tweet}(mID2,"FC", "QC","RC","F","PS","R",idS1),$
$subset_{user}(mID3,"FOLC","FRIC","LC","P","V",idR1),$
$indicator(mID2,mID3,idK),deriveFrom(idS1,idR1,id),rowSums(id,idr1)->$
$rowSums(idS1,idr2),rowSums(idR1,idr3),multi(idK,idr3,idr4),add(idr2,idr4,idr1);$


$user(EID,FOLC,FRIC,LC,P,V),$
$tweetR(EID,FC, QC,RC,F,PS,R),$
$constructMatrix_{11}(mID1,rwID,FOLC,FRIC,LC,P,V,FC,QC,RC,F,PS,R)->$
$nameI(mID1,n),$
$name(mID2,"tweet"),$
$name(mID3,"user"),$
$subset_{tweet}(mID2,"FC", "QC","RC","F","PS","R",idS1),$
$subset_{user}(mID3,"FOLC","FRIC","LC","P","V",idR1),$
$indicator(mID2,mID3,idr3),$
$deriveFrom(idS1,idR1,mID1);$

$name(idS,"tweet"),$
$name(idR,"user"),$
$indicator(idS,idR,idK),$
$subset_{tweet}(idS,"FC", "QC","RC","F","PS","R",idS1),$
$subset_{user}(idR,"FOLC","FRIC","LC","P","V",idR1),$
$rowSums(idS1,idr1),$
$rowSums(idR1,idr2),$
$multi(idK,idr2,idr3),$
$add(idr1,idr3,idr4)->name(idr4,"VV1");$

$tweet(id),$
$child_{sp}(id,"tweetID","o",tID),$
$child_{sp}(id,"flevel","o",fID),$
$child_{sp}(id,"entities","o",eID),$
$child_{sp}(eID,"hashtag","o",hID),$
$child_{sp}(hID,"hID","o",hcID),$
$child_{sp}(id,"place","o",pID),$
$child_{sp}(pID,"code","o",cID)->V1(tID,hcID,fID,cID);$

$tweet(id),$
$child_{sp}(id,"tweetID","o",tID),$
$child_{sp}(id,"text","o",text)->$
$V2(idV2),$
$child_{{sj}_{V2}}(idV2,"tweetID","o",tID),$
$child_{{sj}_{V2}}(idV2,"text","o",text);$
\end{lstlisting}

\newpage
\begin{lstlisting}[caption={Forward Constraints Used for Q5},captionpos=b]
#EGDs
$name(id1,n1),name(id2,n1)->id2=id1;$
$tr(id1,idt1),tr(id1,idt2)->idt2=idt1;$
$in(id1,idt1),in(id1,idt2)->idt2=idt1;$
$ins(id1,idt1),ins(id1,idt2)->idt1=idt2;$
$in(id1,idr1),in(idr1,idr3)->idr3=id1;$
$multi(idA,idB,idr1),multi(idA,idB,idr2)->idr2=idr1;$
$multi_s(idA,idB,idr1),multi_s(idA,idB,idr2)->idr2=idr1;$
$det(idA,d1),det(idA,d2)->d2=d1;$
$trace(idA,id1),trace(idA,id2)->id2=id1;$
$add(idA,idB,idr1),add(idA,idB,idr2)->idr1=idr2;$
$size(idA,i1,j1),size(idA,i2,j2)->j2=j1,i2=i1;$
$name(id1,n1),name(id2,n1)->id2=id1;$
$nameI(mID1,n1),nameI(mID1,n2)->n1=n2;$
$add_s(idA,idB,idr1),add_s(idA,idB,idr2)->idr1=idr2;$
$sum(id1,idt1),sum(id1,idt2)->idt2=idt1;$
$rowSums(idA,id1),rowSums(idA,id2)->id2=id1;$
$colSums(idA,id1),colSums(idA,id2)->id2=id1;$
$user(EID, FOLC1,FRIC1,LC1,P1,V1),user(EID, FOLC2,FRIC2,LC2,P2,V2)-> FOLC2=FOLC1,FRIC2=FRIC1,LC2=LC1,P2=P1,V2=V1;$
$constructMatrix_2(rID,mID,v11,v12),constructMatrix_2(rID,mID,v21,v22)-> v21=v11,v22=v12;$
$constructMatrix_4(rID,mID,v11,v12,v13,v14),constructMatrix_4(rID,mID,v21,v22,v23,v24)->v21=v11,v22=v12,v23=v13,v24=v14;$
$constructMatrix_{11}(rID,mID,v11,v12,v13,v14,v15,v16,v17,v18,v19,v110,v111), constructMatrix_{11}(rID,mID,v21,v22,v23,v24,v25,v26,v27,v28,v29,v210,v211)->$
$v11=v21,v12=v22,v13=vv23,v14=v24,v15=v25,v16=v26,v17=v27,v18=v28,v19=v29,v110=v210,v111=v211;$
$constructMtxMatrix(i,j,v,id)(i1,j1,v1,id),constructMtxMatrix(i2,j2,v2,id)-> i2=i1,j2=j1,v2=v1;$
$indicator(id1,id2,idr31),indicator(id1,id2,idr32)->idr32=idr31;$
$deriveFrom(id1,id2,idr31),deriveFrom(id1,id2,idr32)-> idr32=idr31;$
$concat(id1,id2,idr1),concat(id1,id2,idr2)->idr2=idr1;$
$subset_{tweet}(id1,id2,id3,id4,id5,id6,id7,idr1),$
$subset_{tweet}(id1,id2,id3,id4,id5,id6,id7,idr2)->idr2=idr1;$
$subset_{user}(id1,id2,id3,id4,id5,id6,idr1),$
$subset_{user}(id1,id2,id3,id4,id5,id6,idr2)->idr2=idr1;$
$tweet(id1),tweet(id2)->id2=id1;$
$child_{sp}(x,y1,z,d),child_{sp}(x,y2,z,d)->y2=y1;$
$val_{sp}(x,v1),val_{sp}(x,v2)->v2=v1;$
$child_{{sj}_{V2}}(x,y1,z,d),child_{{sj}_{V2}}(x,y2,z,d)->y2=y1;$

#TGDs
$add(idA,idB,idr1)->add(idB,idA,idr1);$
$multi(id1,id2,idr1),colSums(idr1,idr2)->colSums(id1,idr3),multi(idr3,id2,idr2);$
$multi(id1,id2,idr1),rowSums(idr1,idr2)->rowSums(id2,idr3),multi(id1,idr3,idr2);$
$add(idA,idB,idr1),multi(idr1,idC,idr2)->multi(idA,idC,c1),multi(idB,idC,c2),add(c1,c2,idr2);$
$multi(idA,idB,idr1),multi(idr1,idC,idr2)-> multi(idB,idC,idr3),multi(idA,idr3,idr2);$
$construcMtxMatrix(i,j,v,id),name(id,n),matrixFilterLT(id,x,idr1)->$
$name(idr1,n),construcMtxMatrix(i,j,v,idr1),LT(v,x);$
$add(idA,idB,idr1),multi(idr1,idC,idr2)->multi(idA,idC,c1),multi(idB,idC,c2),add(c1,c2,idr2);$

$subset_{tweet}(mID2,"FC", "QC","RC","F","PS","R",idS1),$
$subset_{user}(mID3,"FOLC","FRIC","LC","P","V",idR1),$
$indicator(mID2,mID3,idK),deriveFrom(idS1,idR1,id),colSums(id,idr1)->$
$colSums(idK,idr2),multi(idr2,idR1,idr3),colSums(idS1,idr4),concat(idr4,idr3,idr1);$


$user(EID,FOLC,FRIC,LC,P,V),$
$tweetR(EID,FC, QC,RC,F,PS,R),$
$constructMatrix_{11}(mID1,rwID,FOLC,FRIC,LC,P,V,FC,QC,RC,F,PS,R)->$
$nameI(mID1,n),$
$name(mID2,"tweet"),$
$name(mID3,"user"),$
$subset_{tweet}(mID2,"FC", "QC","RC","F","PS","R",idS1),$
$subset_{user}(mID3,"FOLC","FRIC","LC","P","V",idR1),$
$indicator(mID2,mID3,idr3),$
$deriveFrom(idS1,idR1,mID1);$
$name(idS,"tweet"),$
$name(idR,"user"),$
$indicator(idS,idR,idK),$
$subset_{tweet}(idS,"FC", "QC","RC","F","PS","R",idS1),$
$subset_{user}(idR,"FOLC","FRIC","LC","P","V",idR1),$
$rowSums(idS1,idr1),$
$rowSums(idR1,idr2),$
$multi(idK,idr2,idr3),$
$add(idr1,idr3,idr4)->name(idr4,"VV1");$

$tweet(id),$
$child_{sp}(id,"tweetID","o",tID),$
$child_{sp}(id,"flevel","o",fID),$
$child_{sp}(id,"entities","o",eID),$
$child_{sp}(eID,"hashtag","o",hID),$
$child_{sp}(hID,"hID","o",hcID),$
$child_{sp}(id,"place","o",pID),$
$child_{sp}(pID,"code","o",cID)->V1(tID,hcID,fID,cID);$

$tweet(id),$
$child_{sp}(id,"tweetID","o",tID),$
$child_{sp}(id,"text","o",text)->$
$V2(idV2),$
$child_{{sj}_{V2}}(idV2,"tweetID","o",tID),$
$child_{{sj}_{V2}}(idV2,"text","o",text);$
\end{lstlisting}

\newpage
\begin{lstlisting}[caption={Forward Constraints Used for Q6},captionpos=b]
#EGDs
$name(id1,n1),name(id2,n1)->id2=id1;$
$tr(id1,idt1),tr(id1,idt2)->idt2=idt1;$
$in(id1,idt1),in(id1,idt2)->idt2=idt1;$
$ins(id1,idt1),ins(id1,idt2)->idt1=idt2;$
$in(id1,idr1),in(idr1,idr3)->idr3=id1;$
$multi(idA,idB,idr1),multi(idA,idB,idr2)->idr2=idr1;$
$multi_s(idA,idB,idr1),multi_s(idA,idB,idr2)->idr2=idr1;$
$det(idA,d1),det(idA,d2)->d2=d1;$
$trace(idA,id1),trace(idA,id2)->id2=id1;$
$add(idA,idB,idr1),add(idA,idB,idr2)->idr1=idr2;$
$size(idA,i1,j1),size(idA,i2,j2)->j2=j1,i2=i1;$
$name(id1,n1),name(id2,n1)->id2=id1;$
$nameI(mID1,n1),nameI(mID1,n2)->n1=n2;$
$add_s(idA,idB,idr1),add_s(idA,idB,idr2)->idr1=idr2;$
$sum(id1,idt1),sum(id1,idt2)->idt2=idt1;$
$rowSums(idA,id1),rowSums(idA,id2)->id2=id1;$
$colSums(idA,id1),colSums(idA,id2)->id2=id1;$
$user(EID, FOLC1,FRIC1,LC1,P1,V1),user(EID, FOLC2,FRIC2,LC2,P2,V2)-> FOLC2=FOLC1,FRIC2=FRIC1,LC2=LC1,P2=P1,V2=V1;$
$constructMatrix_2(rID,mID,v11,v12),constructMatrix_2(rID,mID,v21,v22)-> v21=v11,v22=v12;$
$constructMatrix_4(rID,mID,v11,v12,v13,v14),constructMatrix_4(rID,mID,v21,v22,v23,v24)->v21=v11,v22=v12,v23=v13,v24=v14;$
$constructMatrix_{11}(rID,mID,v11,v12,v13,v14,v15,v16,v17,v18,v19,v110,v111), constructMatrix_{11}(rID,mID,v21,v22,v23,v24,v25,v26,v27,v28,v29,v210,v211)->$
$v11=v21,v12=v22,v13=vv23,v14=v24,v15=v25,v16=v26,v17=v27,v18=v28,v19=v29,v110=v210,v111=v211;$
$constructMtxMatrix(i,j,v,id)(i1,j1,v1,id),constructMtxMatrix(i2,j2,v2,id)-> i2=i1,j2=j1,v2=v1;$
$indicator(id1,id2,idr31),indicator(id1,id2,idr32)->idr32=idr31;$
$deriveFrom(id1,id2,idr31),deriveFrom(id1,id2,idr32)-> idr32=idr31;$
$concat(id1,id2,idr1),concat(id1,id2,idr2)->idr2=idr1;$
$subset_{tweet}(id1,id2,id3,id4,id5,id6,id7,idr1),$
$subset_{tweet}(id1,id2,id3,id4,id5,id6,id7,idr2)->idr2=idr1;$
$subset_{user}(id1,id2,id3,id4,id5,id6,idr1),$
$subset_{user}(id1,id2,id3,id4,id5,id6,idr2)->idr2=idr1;$
$tweet(id1),tweet(id2)->id2=id1;$
$child_{sp}(x,y1,z,d),child_{sp}(x,y2,z,d)->y2=y1;$
$val_{sp}(x,v1),val_{sp}(x,v2)->v2=v1;$
$child_{{sj}_{V2}}(x,y1,z,d),child_{{sj}_{V2}}(x,y2,z,d)->y2=y1;$

#TGDs
$add(idA,idB,idr1)->add(idB,idA,idr1);$
$multi(id1,id2,idr1),colSums(idr1,idr2)->colSums(id1,idr3),multi(idr3,id2,idr2);$
$multi(id1,id2,idr1),rowSums(idr1,idr2)->rowSums(id2,idr3),multi(id1,idr3,idr2);$
$add(idA,idB,idr1),multi(idr1,idC,idr2)->multi(idA,idC,c1),multi(idB,idC,c2),add(c1,c2,idr2);$
$multi(idA,idB,idr1),multi(idr1,idC,idr2)-> multi(idB,idC,idr3),multi(idA,idr3,idr2);$
$construcMtxMatrix(i,j,v,id),name(id,n),matrixFilterLT(id,x,idr1)->$
$name(idr1,n),construcMtxMatrix(i,j,v,idr1),LT(v,x);$
$add(idA,idB,idr1),multi(idr1,idC,idr2)->multi(idA,idC,c1),multi(idB,idC,c2),add(c1,c2,idr2);$

$subset_{tweet}(mID2,"FC", "QC","RC","F","PS","R",idS1),$
$subset_{user}(mID3,"FOLC","FRIC","LC","P","V",idR1),$
$indicator(mID2,mID3,idK),deriveFrom(idS1,idR1,id),colSums(id,idr1)->$
$colSums(idK,idr2),multi(idr2,idR1,idr3),colSums(idS1,idr4),concat(idr4,idr3,idr1);$


$user(EID,FOLC,FRIC,LC,P,V),$
$tweetR(EID,FC, QC,RC,F,PS,R),$
$constructMatrix_{11}(mID1,rwID,FOLC,FRIC,LC,P,V,FC,QC,RC,F,PS,R)->$
$nameI(mID1,n),$
$name(mID2,"tweet"),$
$name(mID3,"user"),$
$subset_{tweet}(mID2,"FC", "QC","RC","F","PS","R",idS1),$
$subset_{user}(mID3,"FOLC","FRIC","LC","P","V",idR1),$
$indicator(mID2,mID3,idr3),$
$deriveFrom(idS1,idR1,mID1);$
$name(idS,"tweet"),$
$name(idR,"user"),$
$indicator(idS,idR,idK),$
$subset_{tweet}(idS,"FC", "QC","RC","F","PS","R",idS1),$
$subset_{user}(idR,"FOLC","FRIC","LC","P","V",idR1),$
$rowSums(idS1,idr1),$
$rowSums(idR1,idr2),$
$multi(idK,idr2,idr3),$
$add(idr1,idr3,idr4)->name(idr4,"VV1");$

$tweet(id),$
$child_{sp}(id,"tweetID","o",tID),$
$child_{sp}(id,"flevel","o",fID),$
$child_{sp}(id,"entities","o",eID),$
$child_{sp}(eID,"hashtag","o",hID),$
$child_{sp}(hID,"hID","o",hcID),$
$child_{sp}(id,"place","o",pID),$
$child_{sp}(pID,"code","o",cID)->V1(tID,hcID,fID,cID);$

$tweet(id),$
$child_{sp}(id,"tweetID","o",tID),$
$child_{sp}(id,"text","o",text)->$
$V2(idV2),$
$child_{{sj}_{V2}}(idV2,"tweetID","o",tID),$
$child_{{sj}_{V2}}(idV2,"text","o",text);$
\end{lstlisting}

\newpage
\begin{lstlisting}[caption={Forward Constraints Used for Q7},captionpos=b]
#EGDs
$name(id1,n1),name(id2,n1)->id2=id1;$
$tr(id1,idt1),tr(id1,idt2)->idt2=idt1;$
$in(id1,idt1),in(id1,idt2)->idt2=idt1;$
$ins(id1,idt1),ins(id1,idt2)->idt1=idt2;$
$in(id1,idr1),in(idr1,idr3)->idr3=id1;$
$multi(idA,idB,idr1),multi(idA,idB,idr2)->idr2=idr1;$
$multi_s(idA,idB,idr1),multi_s(idA,idB,idr2)->idr2=idr1;$
$det(idA,d1),det(idA,d2)->d2=d1;$
$trace(idA,id1),trace(idA,id2)->id2=id1;$
$add(idA,idB,idr1),add(idA,idB,idr2)->idr1=idr2;$
$size(idA,i1,j1),size(idA,i2,j2)->j2=j1,i2=i1;$
$name(id1,n1),name(id2,n1)->id2=id1;$
$nameI(mID1,n1),nameI(mID1,n2)->n1=n2;$
$add_s(idA,idB,idr1),add_s(idA,idB,idr2)->idr1=idr2;$
$sum(id1,idt1),sum(id1,idt2)->idt2=idt1;$
$rowSums(idA,id1),rowSums(idA,id2)->id2=id1;$
$colSums(idA,id1),colSums(idA,id2)->id2=id1;$
$user(EID, FOLC1,FRIC1,LC1,P1,V1),user(EID, FOLC2,FRIC2,LC2,P2,V2)-> FOLC2=FOLC1,FRIC2=FRIC1,LC2=LC1,P2=P1,V2=V1;$
$constructMatrix_2(rID,mID,v11,v12),constructMatrix_2(rID,mID,v21,v22)-> v21=v11,v22=v12;$
$constructMatrix_4(rID,mID,v11,v12,v13,v14),constructMatrix_4(rID,mID,v21,v22,v23,v24)->v21=v11,v22=v12,v23=v13,v24=v14;$
$constructMatrix_{11}(rID,mID,v11,v12,v13,v14,v15,v16,v17,v18,v19,v110,v111), constructMatrix_{11}(rID,mID,v21,v22,v23,v24,v25,v26,v27,v28,v29,v210,v211)->$
$v11=v21,v12=v22,v13=vv23,v14=v24,v15=v25,v16=v26,v17=v27,v18=v28,v19=v29,v110=v210,v111=v211;$
$constructMtxMatrix(i,j,v,id)(i1,j1,v1,id),constructMtxMatrix(i2,j2,v2,id)-> i2=i1,j2=j1,v2=v1;$
$indicator(id1,id2,idr31),indicator(id1,id2,idr32)->idr32=idr31;$
$deriveFrom(id1,id2,idr31),deriveFrom(id1,id2,idr32)-> idr32=idr31;$
$concat(id1,id2,idr1),concat(id1,id2,idr2)->idr2=idr1;$
$subset_{tweet}(id1,id2,id3,id4,id5,id6,id7,idr1),$
$subset_{tweet}(id1,id2,id3,id4,id5,id6,id7,idr2)->idr2=idr1;$
$subset_{user}(id1,id2,id3,id4,id5,id6,idr1),$
$subset_{user}(id1,id2,id3,id4,id5,id6,idr2)->idr2=idr1;$
$tweet(id1),tweet(id2)->id2=id1;$
$child_{sp}(x,y1,z,d),child_{sp}(x,y2,z,d)->y2=y1;$
$val_{sp}(x,v1),val_{sp}(x,v2)->v2=v1;$
$child_{{sj}_{V2}}(x,y1,z,d),child_{{sj}_{V2}}(x,y2,z,d)->y2=y1;$

#TGDs
$add(idA,idB,idr1)->add(idB,idA,idr1);$
$multi(idA,idB,idr1),multi(idr1,idC,idr2)-> multi(idB,idC,idr3),multi(idA,idr3,idr2);$
$multi(id1,id2,idr1),colSums(idr1,idr2)->colSums(id1,idr3),multi(idr3,id2,idr2);$
$multi(id1,id2,idr1),rowSums(idr1,idr2)->rowSums(id2,idr3),multi(id1,idr3,idr2);$
$add(idA,idB,idr1),multi(idr1,idC,idr2)->multi(idA,idC,c1),multi(idB,idC,c2),add(c1,c2,idr2);$
$construcMtxMatrix(i,j,v,id),name(id,n),matrixFilterLT(id,x,idr1)->$
$name(idr1,n),construcMtxMatrix(i,j,v,idr1),LT(v,x);$
$add(idA,idB,idr1),multi(idr1,idC,idr2)->multi(idA,idC,c1),multi(idB,idC,c2),add(c1,c2,idr2);$

$subset_{tweet}(mID2,"FC", "QC","RC","F","PS","R",idS1),$
$subset_{user}(mID3,"FOLC","FRIC","LC","P","V",idR1),$
$indicator(mID2,mID3,idK),deriveFrom(idS1,idR1,id),colSums(id,idr1)->$
$colSums(idK,idr2),multi(idr2,idR1,idr3),colSums(idS1,idr4),concat(idr4,idr3,idr1);$


$user(EID,FOLC,FRIC,LC,P,V),$
$tweetR(EID,FC, QC,RC,F,PS,R),$
$constructMatrix_{11}(mID1,rwID,FOLC,FRIC,LC,P,V,FC,QC,RC,F,PS,R)->$
$nameI(mID1,n),$
$name(mID2,"tweet"),$
$name(mID3,"user"),$
$subset_{tweet}(mID2,"FC", "QC","RC","F","PS","R",idS1),$
$subset_{user}(mID3,"FOLC","FRIC","LC","P","V",idR1),$
$indicator(mID2,mID3,idr3),$
$deriveFrom(idS1,idR1,mID1);$

$name(idS,"tweet"),$
$name(idR,"user"),$
$indicator(idS,idR,idK),$
$subset_{tweet}(idS,"FC", "QC","RC","F","PS","R",idS1),$
$subset_{user}(idR,"FOLC","FRIC","LC","P","V",idR1),$
$rowSums(idS1,idr1),$
$rowSums(idR1,idr2),$
$multi(idK,idr2,idr3),$
$add(idr1,idr3,idr4)->name(idr4,"VV1");$

$tweet(id),$
$child_{sp}(id,"tweetID","o",tID),$
$child_{sp}(id,"flevel","o",fID),$
$child_{sp}(id,"entities","o",eID),$
$child_{sp}(eID,"hashtag","o",hID),$
$child_{sp}(hID,"hID","o",hcID),$
$child_{sp}(id,"place","o",pID),$
$child_{sp}(pID,"code","o",cID)->V1(tID,hcID,fID,cID);$

$tweet(id),$
$child_{sp}(id,"tweetID","o",tID),$
$child_{sp}(id,"text","o",text)->$
$V2(idV2),$
$child_{{sj}_{V2}}(idV2,"tweetID","o",tID),$
$child_{{sj}_{V2}}(idV2,"text","o",text);$
\end{lstlisting}

\newpage
\begin{lstlisting}[caption={Forward Constraints Used for Q8},captionpos=b]
#EGDs
$name(id1,n1),name(id2,n1)->id2=id1;$
$tr(id1,idt1),tr(id1,idt2)->idt2=idt1;$
$in(id1,idt1),in(id1,idt2)->idt2=idt1;$
$ins(id1,idt1),ins(id1,idt2)->idt1=idt2;$
$in(id1,idr1),in(idr1,idr3)->idr3=id1;$
$multi(idA,idB,idr1),multi(idA,idB,idr2)->idr2=idr1;$
$multi_s(idA,idB,idr1),multi_s(idA,idB,idr2)->idr2=idr1;$
$det(idA,d1),det(idA,d2)->d2=d1;$
$trace(idA,id1),trace(idA,id2)->id2=id1;$
$add(idA,idB,idr1),add(idA,idB,idr2)->idr1=idr2;$
$size(idA,i1,j1),size(idA,i2,j2)->j2=j1,i2=i1;$
$name(id1,n1),name(id2,n1)->id2=id1;$
$nameI(mID1,n1),nameI(mID1,n2)->n1=n2;$
$add_s(idA,idB,idr1),add_s(idA,idB,idr2)->idr1=idr2;$
$sum(id1,idt1),sum(id1,idt2)->idt2=idt1;$
$rowSums(idA,id1),rowSums(idA,id2)->id2=id1;$
$colSums(idA,id1),colSums(idA,id2)->id2=id1;$
$user(EID, FOLC1,FRIC1,LC1,P1,V1),user(EID, FOLC2,FRIC2,LC2,P2,V2)-> FOLC2=FOLC1,FRIC2=FRIC1,LC2=LC1,P2=P1,V2=V1;$
$constructMatrix_2(rID,mID,v11,v12),constructMatrix_2(rID,mID,v21,v22)-> v21=v11,v22=v12;$
$constructMatrix_4(rID,mID,v11,v12,v13,v14),constructMatrix_4(rID,mID,v21,v22,v23,v24)->v21=v11,v22=v12,v23=v13,v24=v14;$
$constructMatrix_{11}(rID,mID,v11,v12,v13,v14,v15,v16,v17,v18,v19,v110,v111), constructMatrix_{11}(rID,mID,v21,v22,v23,v24,v25,v26,v27,v28,v29,v210,v211)->$
$v11=v21,v12=v22,v13=vv23,v14=v24,v15=v25,v16=v26,v17=v27,v18=v28,v19=v29,v110=v210,v111=v211;$
$constructMtxMatrix(i,j,v,id)(i1,j1,v1,id),constructMtxMatrix(i2,j2,v2,id)-> i2=i1,j2=j1,v2=v1;$
$indicator(id1,id2,idr31),indicator(id1,id2,idr32)->idr32=idr31;$
$deriveFrom(id1,id2,idr31),deriveFrom(id1,id2,idr32)-> idr32=idr31;$
$concat(id1,id2,idr1),concat(id1,id2,idr2)->idr2=idr1;$
$subset_{tweet}(id1,id2,id3,id4,id5,id6,id7,idr1),$
$subset_{tweet}(id1,id2,id3,id4,id5,id6,id7,idr2)->idr2=idr1;$
$subset_{user}(id1,id2,id3,id4,id5,id6,idr1),$
$subset_{user}(id1,id2,id3,id4,id5,id6,idr2)->idr2=idr1;$
$tweet(id1),tweet(id2)->id2=id1;$
$child_{sp}(x,y1,z,d),child_{sp}(x,y2,z,d)->y2=y1;$
$val_{sp}(x,v1),val_{sp}(x,v2)->v2=v1;$
$child_{{sj}_{V2}}(x,y1,z,d),child_{{sj}_{V2}}(x,y2,z,d)->y2=y1;$

#TGDs
$add(idA,idB,idr1)->add(idB,idA,idr1);$
$multi(id1,id2,idr1),colSums(idr1,idr2)->colSums(id1,idr3),multi(idr3,id2,idr2);$
$multi(idA,idB,idr1),multi(idr1,idC,idr2)-> multi(idB,idC,idr3),multi(idA,idr3,idr2);$
$add(idA,idB,idr1),multi(idr1,idC,idr2)->multi(idA,idC,c1),multi(idB,idC,c2),add(c1,c2,idr2);$
$add(idA,idB,idr1),trace(idr1,t)->trace(idA,idr2),trace(idB,idr3),add_s(idr2,idr3,t);$

$construcMtxMatrix(i,j,v,id),name(id,n),matrixFilterLT(id,x,idr1)->$
$name(idr1,n),construcMtxMatrix(i,j,v,idr1),LT(v,x);$
$add(idA,idB,idr1),multi(idr1,idC,idr2)->multi(idA,idC,c1),multi(idB,idC,c2),add(c1,c2,idr2);$

$subset_{tweet}(mID2,"FC", "QC","RC","F","PS","R",idS1),$
$subset_{user}(mID3,"FOLC","FRIC","LC","P","V",idR1),$
$indicator(mID2,mID3,idK),deriveFrom(idS1,idR1,id),colSums(id,idr1)->$
$colSums(idK,idr2),multi(idr2,idR1,idr3),colSums(idS1,idr4),concat(idr4,idr3,idr1);$


$user(EID,FOLC,FRIC,LC,P,V),$
$tweetR(EID,FC, QC,RC,F,PS,R),$
$constructMatrix_{11}(mID1,rwID,FOLC,FRIC,LC,P,V,FC,QC,RC,F,PS,R)->$
$nameI(mID1,n),$
$name(mID2,"tweet"),$
$name(mID3,"user"),$
$subset_{tweet}(mID2,"FC", "QC","RC","F","PS","R",idS1),$
$subset_{user}(mID3,"FOLC","FRIC","LC","P","V",idR1),$
$indicator(mID2,mID3,idr3),$
$deriveFrom(idS1,idR1,mID1);$

$name(idS,"tweet"),$
$name(idR,"user"),$
$indicator(idS,idR,idK),$
$subset_{tweet}(idS,"FC", "QC","RC","F","PS","R",idS1),$
$subset_{user}(idR,"FOLC","FRIC","LC","P","V",idR1),$
$rowSums(idS1,idr1),$
$rowSums(idR1,idr2),$
$multi(idK,idr2,idr3),$
$add(idr1,idr3,idr4)->name(idr4,"VV1");$

$tweet(id),$
$child_{sp}(id,"tweetID","o",tID),$
$child_{sp}(id,"flevel","o",fID),$
$child_{sp}(id,"entities","o",eID),$
$child_{sp}(eID,"hashtag","o",hID),$
$child_{sp}(hID,"hID","o",hcID),$
$child_{sp}(id,"place","o",pID),$
$child_{sp}(pID,"code","o",cID)->V1(tID,hcID,fID,cID);$

$tweet(id),$
$child_{sp}(id,"tweetID","o",tID),$
$child_{sp}(id,"text","o",text)->$
$V2(idV2),$
$child_{{sj}_{V2}}(idV2,"tweetID","o",tID),$
$child_{{sj}_{V2}}(idV2,"text","o",text);$
\end{lstlisting}

\newpage
\begin{lstlisting}[caption={Forward Constraints Used for Q9},captionpos=b]
#EGDs
$name(id1,n1),name(id2,n1)->id2=id1;$
$tr(id1,idt1),tr(id1,idt2)->idt2=idt1;$
$in(id1,idt1),in(id1,idt2)->idt2=idt1;$
$ins(id1,idt1),ins(id1,idt2)->idt1=idt2;$
$in(id1,idr1),in(idr1,idr3)->idr3=id1;$
$multi(idA,idB,idr1),multi(idA,idB,idr2)->idr2=idr1;$
$multi_s(idA,idB,idr1),multi_s(idA,idB,idr2)->idr2=idr1;$
$det(idA,d1),det(idA,d2)->d2=d1;$
$trace(idA,id1),trace(idA,id2)->id2=id1;$
$add(idA,idB,idr1),add(idA,idB,idr2)->idr1=idr2;$
$size(idA,i1,j1),size(idA,i2,j2)->j2=j1,i2=i1;$
$name(id1,n1),name(id2,n1)->id2=id1;$
$nameI(mID1,n1),nameI(mID1,n2)->n1=n2;$
$add_s(idA,idB,idr1),add_s(idA,idB,idr2)->idr1=idr2;$
$sum(id1,idt1),sum(id1,idt2)->idt2=idt1;$
$rowSums(idA,id1),rowSums(idA,id2)->id2=id1;$
$colSums(idA,id1),colSums(idA,id2)->id2=id1;$
$user(EID, FOLC1,FRIC1,LC1,P1,V1),user(EID, FOLC2,FRIC2,LC2,P2,V2)-> FOLC2=FOLC1,FRIC2=FRIC1,LC2=LC1,P2=P1,V2=V1;$
$constructMatrix_2(rID,mID,v11,v12),constructMatrix_2(rID,mID,v21,v22)-> v21=v11,v22=v12;$
$constructMatrix_4(rID,mID,v11,v12,v13,v14),constructMatrix_4(rID,mID,v21,v22,v23,v24)->v21=v11,v22=v12,v23=v13,v24=v14;$
$constructMatrix_{11}(rID,mID,v11,v12,v13,v14,v15,v16,v17,v18,v19,v110,v111), constructMatrix_{11}(rID,mID,v21,v22,v23,v24,v25,v26,v27,v28,v29,v210,v211)->$
$v11=v21,v12=v22,v13=vv23,v14=v24,v15=v25,v16=v26,v17=v27,v18=v28,v19=v29,v110=v210,v111=v211;$
$constructMtxMatrix(i,j,v,id)(i1,j1,v1,id),constructMtxMatrix(i2,j2,v2,id)-> i2=i1,j2=j1,v2=v1;$
$indicator(id1,id2,idr31),indicator(id1,id2,idr32)->idr32=idr31;$
$deriveFrom(id1,id2,idr31),deriveFrom(id1,id2,idr32)-> idr32=idr31;$
$concat(id1,id2,idr1),concat(id1,id2,idr2)->idr2=idr1;$
$subset_{tweet}(id1,id2,id3,id4,id5,id6,id7,idr1),$
$subset_{tweet}(id1,id2,id3,id4,id5,id6,id7,idr2)->idr2=idr1;$
$subset_{user}(id1,id2,id3,id4,id5,id6,idr1),$
$subset_{user}(id1,id2,id3,id4,id5,id6,idr2)->idr2=idr1;$
$tweet(id1),tweet(id2)->id2=id1;$
$child_{sp}(x,y1,z,d),child_{sp}(x,y2,z,d)->y2=y1;$
$val_{sp}(x,v1),val_{sp}(x,v2)->v2=v1;$
$child_{{sj}_{V2}}(x,y1,z,d),child_{{sj}_{V2}}(x,y2,z,d)->y2=y1;$

#TGDs
$colSums(id1,idr1),tr(idr1,idr2),rowSums(id2,idr3),multi_e(idr2,idr3,idr4),sum(idr4,s)->$
$multi(id1,id2,idr5),sum(idr5,s);$
$multi(id1,id2,idr1),colSums(idr1,idr2)->colSums(id1,idr3),multi(idr3,id2,idr2);$
$multi(idA,idB,idr1),multi(idr1,idC,idr2)-> multi(idB,idC,idr3),multi(idA,idr3,idr2);$
$construcMtxMatrix(i,j,v,id),name(id,n),matrixFilterLT(id,x,idr1)->$
$name(idr1,n),construcMtxMatrix(i,j,v,idr1),LT(v,x);$
$add(idA,idB,idr1),multi(idr1,idC,idr2)->multi(idA,idC,c1),multi(idB,idC,c2),add(c1,c2,idr2);$

$subset_{tweet}(mID2,"FC", "QC","RC","F","PS","R",idS1),$
$subset_{user}(mID3,"FOLC","FRIC","LC","P","V",idR1),$
$indicator(mID2,mID3,idK),deriveFrom(idS1,idR1,id),$
$multi(idX,id,idr1)->$
$multi(idX,idK,idr2),$
$multi(idr2,idR1,idr3),$
$multi(idX,idS1,idr4),$
$concat(idr4,idr3,idr1);$

$user(EID,FOLC,FRIC,LC,P,V),$
$tweetR(EID,FC, QC,RC,F,PS,R),$
$constructMatrix_{11}(mID1,rwID,FOLC,FRIC,LC,P,V,FC,QC,RC,F,PS,R)->$
$nameI(mID1,n),$
$name(mID2,"tweet"),$
$name(mID3,"user"),$
$subset_{tweet}(mID2,"FC", "QC","RC","F","PS","R",idS1),$
$subset_{user}(mID3,"FOLC","FRIC","LC","P","V",idR1),$
$indicator(mID2,mID3,idr3),$
$deriveFrom(idS1,idR1,mID1);$

$name(idS,"tweet"),$
$name(idR,"user"),$
$indicator(idS,idR,idK),$
$subset_{tweet}(idS,"FC", "QC","RC","F","PS","R",idS1),$
$subset_{user}(idR,"FOLC","FRIC","LC","P","V",idR1),$
$name(idC,"C"),$
$multi(idC,idK,idr1),$
$multi(idr1,idR1,idr3),$
$multi(idC,idS1,idr4),$
$concat(idr4,idr3,idr5)->name(idr5,"VV1");$

$tweet(id),$
$child_{sp}(id,"tweetID","o",tID),$
$child_{sp}(id,"flevel","o",fID),$
$child_{sp}(id,"entities","o",eID),$
$child_{sp}(eID,"hashtag","o",hID),$
$child_{sp}(hID,"hID","o",hcID),$
$child_{sp}(id,"place","o",pID),$
$child_{sp}(pID,"code","o",cID)->V1(tID,hcID,fID,cID);$

$tweet(id),$
$child_{sp}(id,"tweetID","o",tID),$
$child_{sp}(id,"text","o",text)->$
$V2(idV2),$
$child_{{sj}_{V2}}(idV2,"tweetID","o",tID),$
$child_{{sj}_{V2}}(idV2,"text","o",text);$
\end{lstlisting}

\newpage
\begin{lstlisting}[caption={Forward Constraints Used for Q10},captionpos=b]
#EGDs
$name(id1,n1),name(id2,n1)->id2=id1;$
$tr(id1,idt1),tr(id1,idt2)->idt2=idt1;$
$in(id1,idt1),in(id1,idt2)->idt2=idt1;$
$ins(id1,idt1),ins(id1,idt2)->idt1=idt2;$
$in(id1,idr1),in(idr1,idr3)->idr3=id1;$
$multi(idA,idB,idr1),multi(idA,idB,idr2)->idr2=idr1;$
$multi_s(idA,idB,idr1),multi_s(idA,idB,idr2)->idr2=idr1;$
$det(idA,d1),det(idA,d2)->d2=d1;$
$trace(idA,id1),trace(idA,id2)->id2=id1;$
$add(idA,idB,idr1),add(idA,idB,idr2)->idr1=idr2;$
$size(idA,i1,j1),size(idA,i2,j2)->j2=j1,i2=i1;$
$name(id1,n1),name(id2,n1)->id2=id1;$
$nameI(mID1,n1),nameI(mID1,n2)->n1=n2;$
$add_s(idA,idB,idr1),add_s(idA,idB,idr2)->idr1=idr2;$
$sum(id1,idt1),sum(id1,idt2)->idt2=idt1;$
$rowSums(idA,id1),rowSums(idA,id2)->id2=id1;$
$colSums(idA,id1),colSums(idA,id2)->id2=id1;$
$user(EID, FOLC1,FRIC1,LC1,P1,V1),user(EID, FOLC2,FRIC2,LC2,P2,V2)-> FOLC2=FOLC1,FRIC2=FRIC1,LC2=LC1,P2=P1,V2=V1;$
$constructMatrix_2(rID,mID,v11,v12),constructMatrix_2(rID,mID,v21,v22)-> v21=v11,v22=v12;$
$constructMatrix_4(rID,mID,v11,v12,v13,v14),constructMatrix_4(rID,mID,v21,v22,v23,v24)->v21=v11,v22=v12,v23=v13,v24=v14;$
$constructMatrix_{11}(rID,mID,v11,v12,v13,v14,v15,v16,v17,v18,v19,v110,v111), constructMatrix_{11}(rID,mID,v21,v22,v23,v24,v25,v26,v27,v28,v29,v210,v211)->$
$v11=v21,v12=v22,v13=vv23,v14=v24,v15=v25,v16=v26,v17=v27,v18=v28,v19=v29,v110=v210,v111=v211;$
$constructMtxMatrix(i,j,v,id)(i1,j1,v1,id),constructMtxMatrix(i2,j2,v2,id)-> i2=i1,j2=j1,v2=v1;$
$indicator(id1,id2,idr31),indicator(id1,id2,idr32)->idr32=idr31;$
$deriveFrom(id1,id2,idr31),deriveFrom(id1,id2,idr32)-> idr32=idr31;$
$concat(id1,id2,idr1),concat(id1,id2,idr2)->idr2=idr1;$
$subset_{tweet}(id1,id2,id3,id4,id5,id6,id7,idr1),$
$subset_{tweet}(id1,id2,id3,id4,id5,id6,id7,idr2)->idr2=idr1;$
$subset_{user}(id1,id2,id3,id4,id5,id6,idr1),$
$subset_{user}(id1,id2,id3,id4,id5,id6,idr2)->idr2=idr1;$
$tweet(id1),tweet(id2)->id2=id1;$
$child_{sp}(x,y1,z,d),child_{sp}(x,y2,z,d)->y2=y1;$
$val_{sp}(x,v1),val_{sp}(x,v2)->v2=v1;$
$child_{{sj}_{V2}}(x,y1,z,d),child_{{sj}_{V2}}(x,y2,z,d)->y2=y1;$

#TGDs
$colSums(id1,idr1),tr(idr1,idr2),rowSums(id2,idr3),multi_e(idr2,idr3,idr4),sum(idr4,s)->$
$multi(id1,id2,idr5),sum(idr5,s);$
$multi(id1,id2,idr1),colSums(idr1,idr2)->colSums(id1,idr3),multi(idr3,id2,idr2);$
$multi(idA,idB,idr1),multi(idr1,idC,idr2)-> multi(idB,idC,idr3),multi(idA,idr3,idr2);$
$construcMtxMatrix(i,j,v,id),name(id,n),matrixFilterLT(id,x,idr1)->$
$name(idr1,n),construcMtxMatrix(i,j,v,idr1),LT(v,x);$
$add(idA,idB,idr1),multi(idr1,idC,idr2)->multi(idA,idC,c1),multi(idB,idC,c2),add(c1,c2,idr2);$

$subset_{tweet}(mID2,"FC", "QC","RC","F","PS","R",idS1),$
$subset_{user}(mID3,"FOLC","FRIC","LC","P","V",idR1),$
$indicator(mID2,mID3,idK),deriveFrom(idS1,idR1,id),$
$multi(idX,id,idr1)->$
$multi(idX,idK,idr2),$
$multi(idr2,idR1,idr3),$
$multi(idX,idS1,idr4),$
$concat(idr4,idr3,idr1);$

$user(EID,FOLC,FRIC,LC,P,V),$
$tweetR(EID,FC, QC,RC,F,PS,R),$
$constructMatrix_{11}(mID1,rwID,FOLC,FRIC,LC,P,V,FC,QC,RC,F,PS,R)->$
$nameI(mID1,n),$
$name(mID2,"tweet"),$
$name(mID3,"user"),$
$subset_{tweet}(mID2,"FC", "QC","RC","F","PS","R",idS1),$
$subset_{user}(mID3,"FOLC","FRIC","LC","P","V",idR1),$
$indicator(mID2,mID3,idr3),$
$deriveFrom(idS1,idR1,mID1);$

$name(idS,"tweet"),$
$name(idR,"user"),$
$indicator(idS,idR,idK),$
$subset_{tweet}(idS,"FC", "QC","RC","F","PS","R",idS1),$
$subset_{user}(idR,"FOLC","FRIC","LC","P","V",idR1),$
$name(idC,"C"),$
$multi(idC,idK,idr1),$
$multi(idr1,idR1,idr3),$
$multi(idC,idS1,idr4),$
$concat(idr4,idr3,idr5)->name(idr5,"VV1");$

$tweet(id),$
$child_{sp}(id,"tweetID","o",tID),$
$child_{sp}(id,"flevel","o",fID),$
$child_{sp}(id,"entities","o",eID),$
$child_{sp}(eID,"hashtag","o",hID),$
$child_{sp}(hID,"hID","o",hcID),$
$child_{sp}(id,"place","o",pID),$
$child_{sp}(pID,"code","o",cID)->V1(tID,hcID,fID,cID);$

$tweet(id),$
$child_{sp}(id,"tweetID","o",tID),$
$child_{sp}(id,"text","o",text)->$
$V2(idV2),$
$child_{{sj}_{V2}}(idV2,"tweetID","o",tID),$
$child_{{sj}_{V2}}(idV2,"text","o",text);$
\end{lstlisting}
