# Supplementary material for: HADAD: A Lightweight Approach for Optimizing Hybrid Complex Analytics Queries (Extended Version)
Source: arXiv:2103.12317 source file (2021-03-23)
Supplement: Supplementary file 2 [file appendix2.tex]

\onecolumn
\section{Appendix C}
\begin{table*}[ht]	
\centering	
\begin{tabular}{ |c|c| } 
%\hline
%\multicolumn{2}{|c|}{\textbf{pushdownSumOnAdd}}\\\hline
%sum(A+B) -> sum(A)+sum(B) & $\forall idA,idB, idR1,r $ $ add(idA,idB,idR1), sum(idR1,r) \rightarrow$\\
%						  & $\exists r1, r2$ $sum(idA,r1),sum(idA,r2), add_s(r1,r2,r)$\\
%\hline
%\multicolumn{2}{|c|}{\textbf{pushdownBinaryOperationOnDiag}}\\\hline
%diag(X)*s -> diag(X*s) 	  & $\forall idX,s,r$ $diag(idX,idR1),multi_s(idR1,s,r)\rightarrow \exists idR2 multi_s(idX,s,idR2), diag(idR2,r)$\\
%\hline
%\multicolumn{2}{|c|}{\textbf{simplifySumDiagToTrace}}\\\hline
%sum(diag(X)) -> trace(X)  & $\forall idX, idR1, r $ $diag(idX,idR1),sum(idR1,r) \rightarrow trace(idX,r)$\\
%\hline
%\multicolumn{2}{|c|}{\textbf{EmptyReorgOp}}\\\hline
%t(X)->X if x is a zero matrix &  $\forall idX $ $Zero(idX)->tr(idX,idX)$\\ 
%\hline
%rev(X)->X if x is a zero matrix &  $\forall idX $ $Zero(idX)->rev(idX,idX)$\\
%\hline
%diag(X)->X if x is a zero matrix &  $\forall idX $ $Zero(idX)->diag(idX,idX)$\\
%\hline
\multicolumn{2}{|c|}{\textbf{ColSumsMVMult}}\\\hline
colSums(X*Y) -> t(Y)X & $\forall idX,idY,idR1,r,i$ $size(idY,i,"1"),multi_s(idX,idY,idR1), colSums(idR1,r)$\\
							 & $\exists idYT tr(idY,idYT),multi(idYT,idX,r) $\\
\hline 
rowSums(X*Y) -> Xt(Y)& $\forall idX,idY,idR1,r,i$ $size(idY,"1",i),multi_s(idX,idY,idR1), rowSums(idR1,r)$\\
							 & $\exists idYT tr(idY,idYT),multi(idX,idYT,r) $
\\
\hline
\end{tabular}
\end{table*}
