# Supplementary material for: HADAD: A Lightweight Approach for Optimizing Hybrid Complex Analytics Queries (Extended Version)
Source: arXiv:2103.12317 source file (2021-03-23)
Supplement: Supplementary file 3 [file appendixG.tex]

\onecolumn
\section{Additional Results: Factorized LA Experiments}
\label{appendixG}
\begin{figure*}[!htbp]
\figspa
  \centering
      \subfigure[\textbf{P1.1}]{\includegraphics[scale=0.25,width=5.5cm,height=4.5cm]{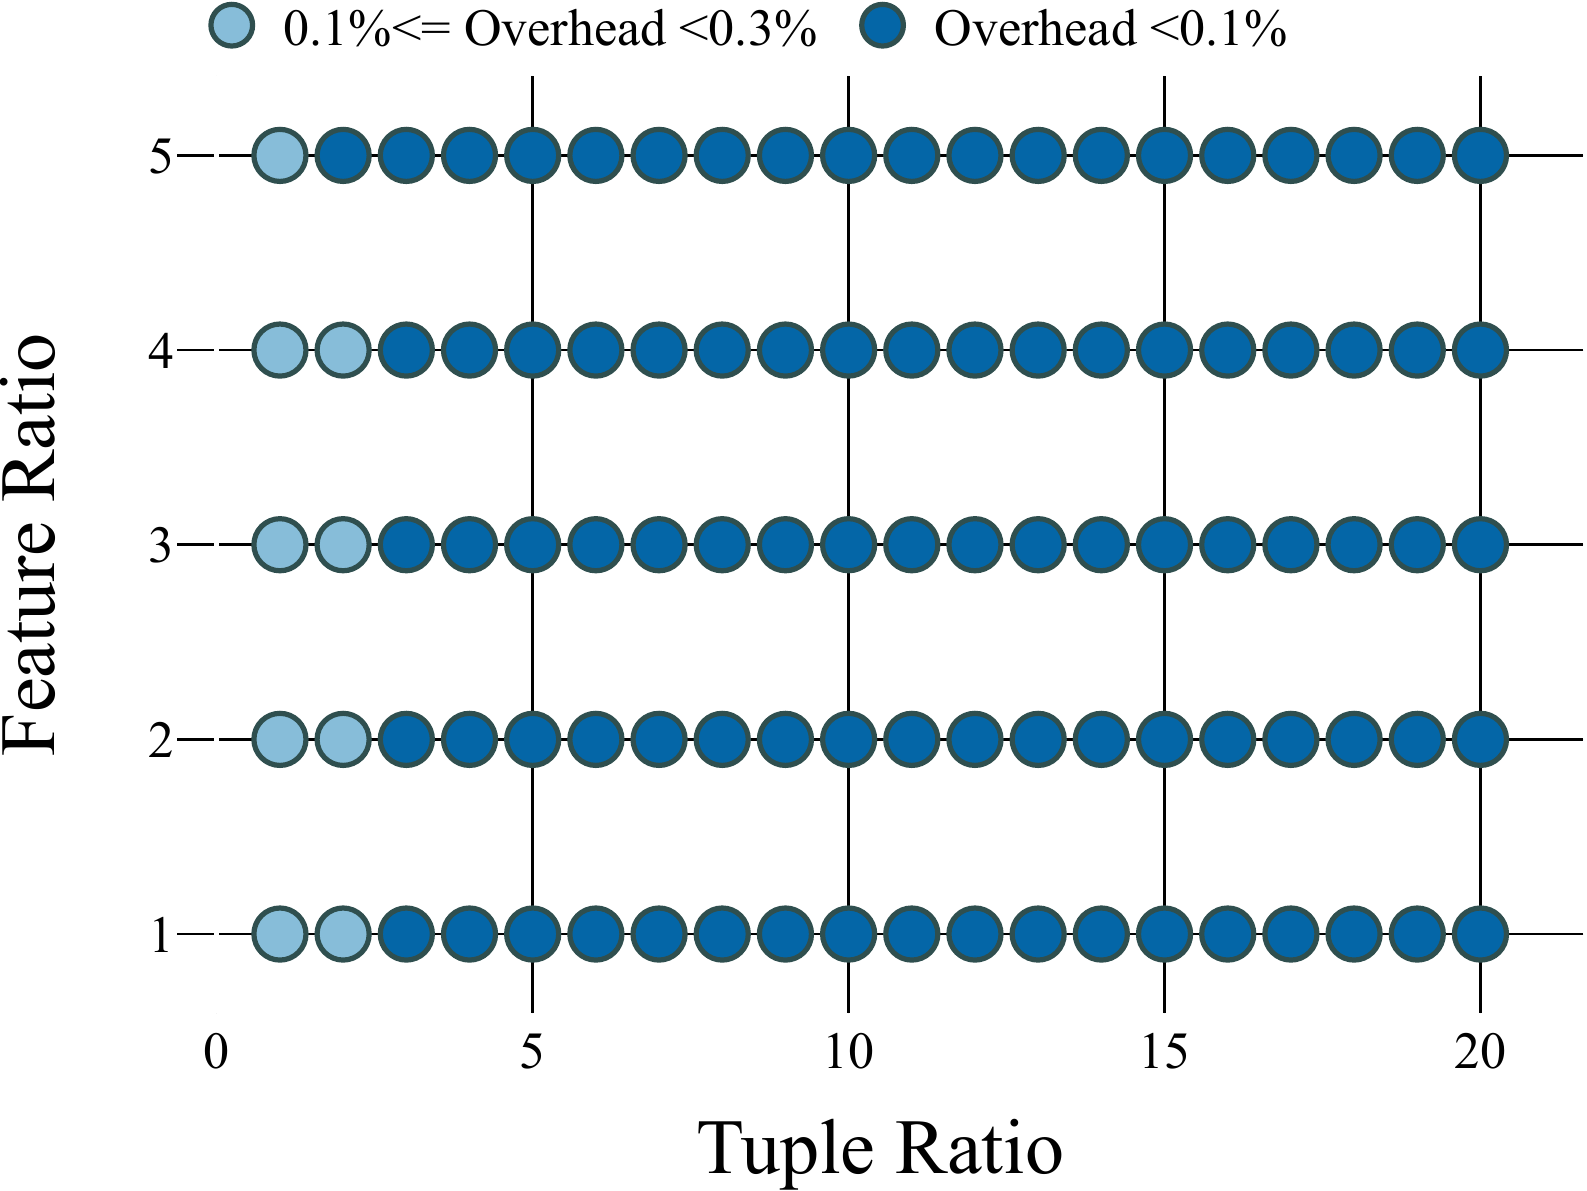}}
      \subfigure[\textbf{P1.10}]{\includegraphics[scale=0.25,width=5.5cm,height=4.5cm]{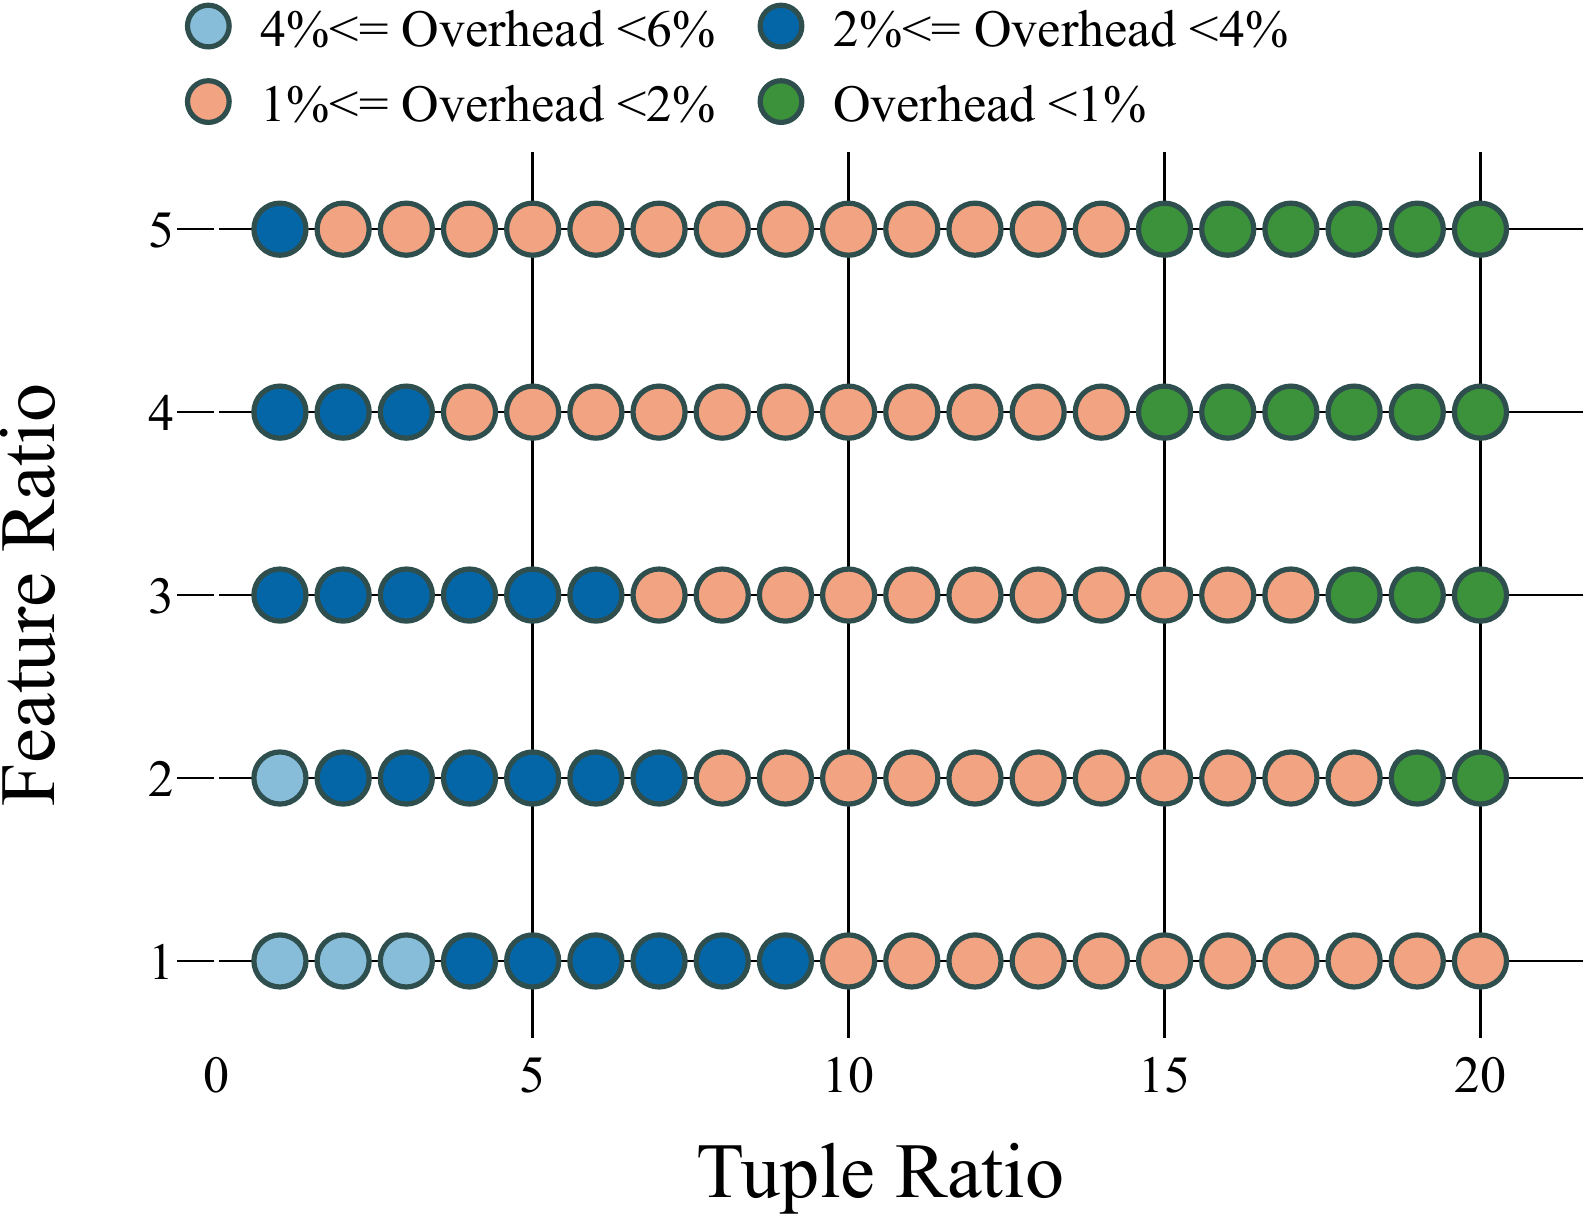}}
      \subfigure[\textbf{P1.13}]{\includegraphics[scale=0.25,width=5.5cm,height=4.5cm]{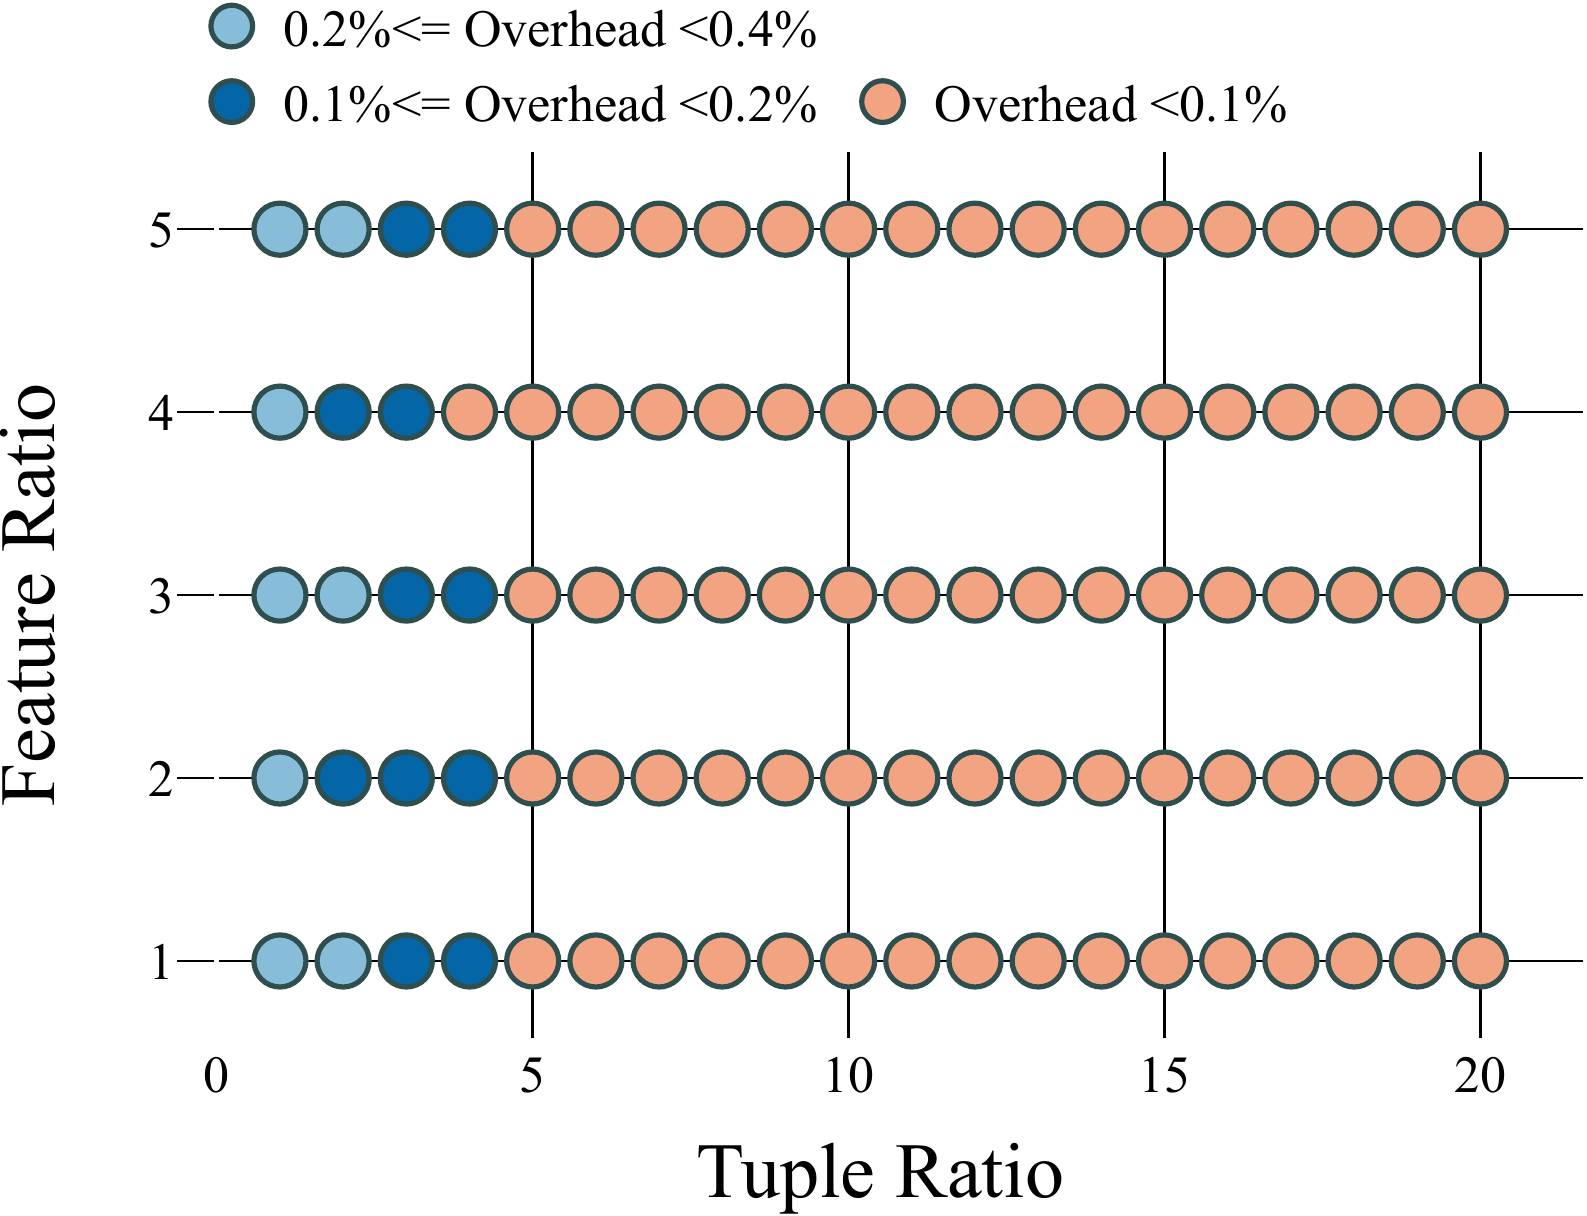}}
 \figspb\figspb\figspb
 \caption{HADAD $RW_{find}$ overhead as a percentage (\%) of the total time ($Q_{exec}+ RW_{fond}$) for pipelines 1.1,1.10 and 1.13 running on MorpheusR}
 \figspc 
 \label{fig:la-overhead-1}
\end{figure*}
 \figspc
\begin{figure*}[!htbp]
\figspa
  \centering
      \subfigure[\textbf{P1.16}]{\includegraphics[scale=0.25,width=5.5cm,height=4.5cm]{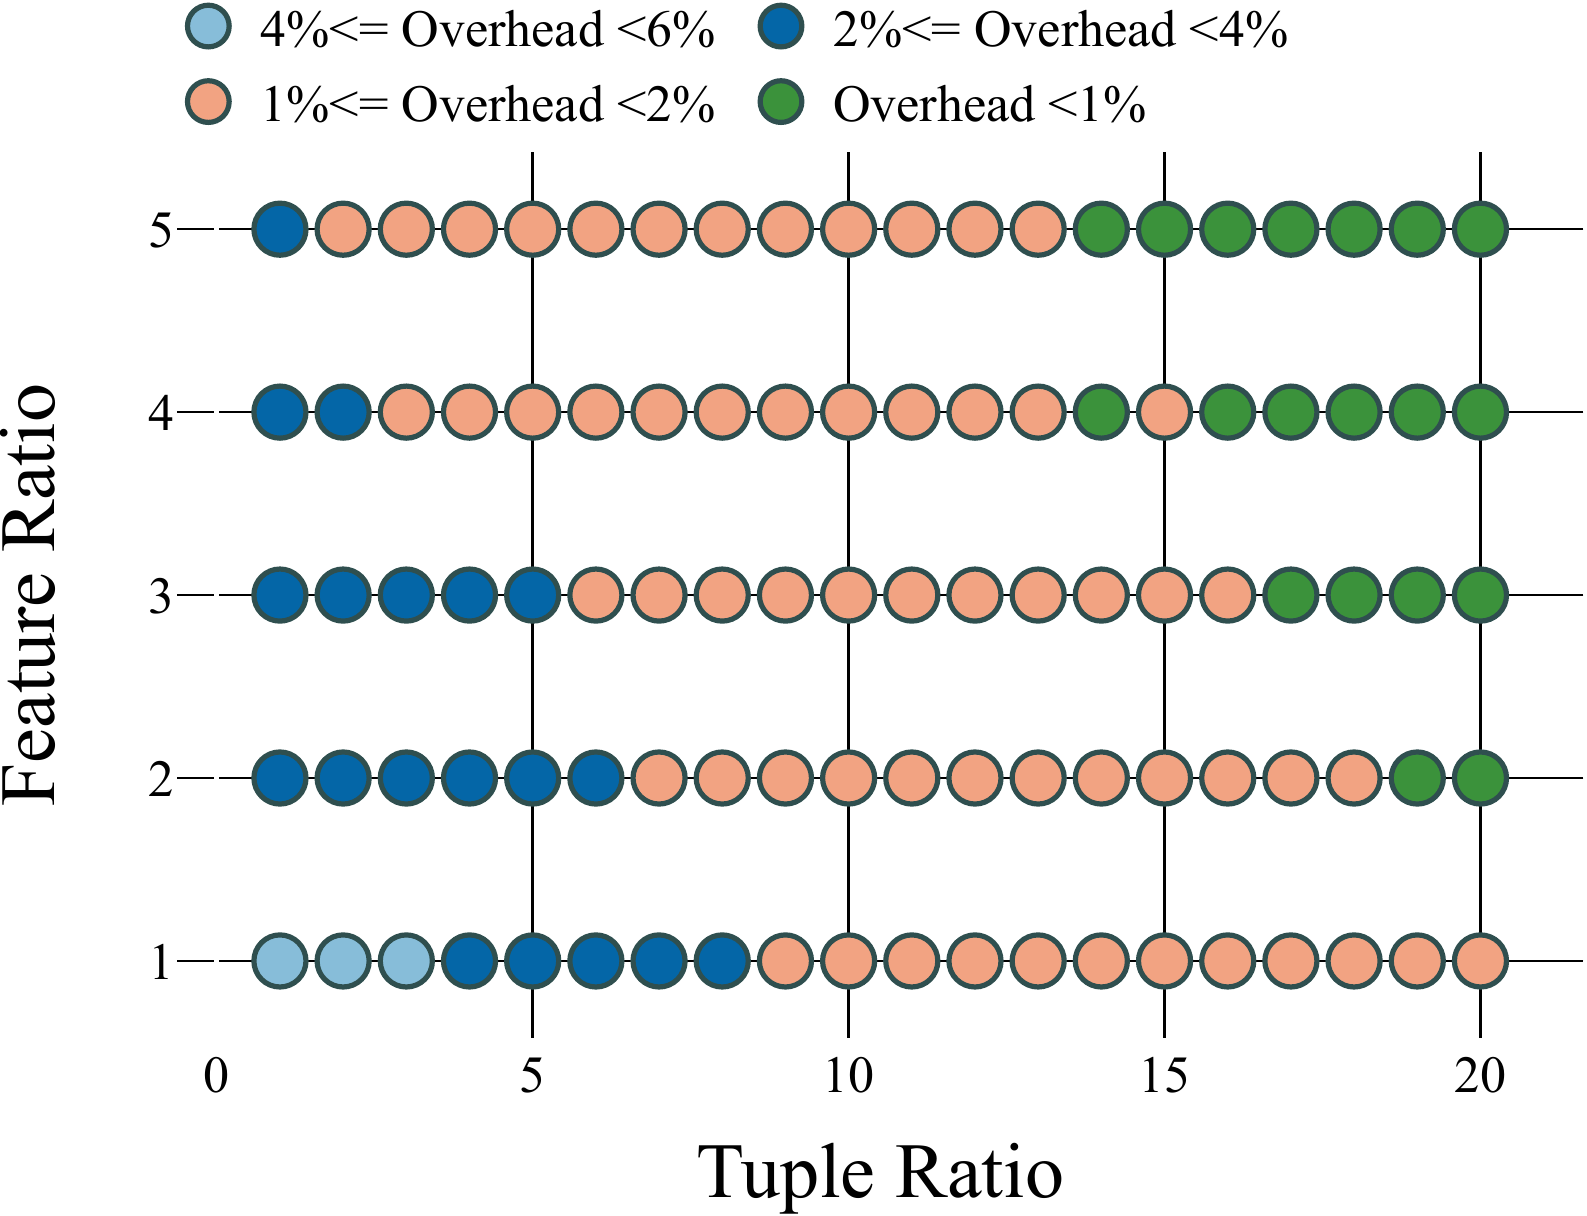}}
      \subfigure[\textbf{P1.18}]{\includegraphics[scale=0.25,width=5.5cm,height=4.5cm]{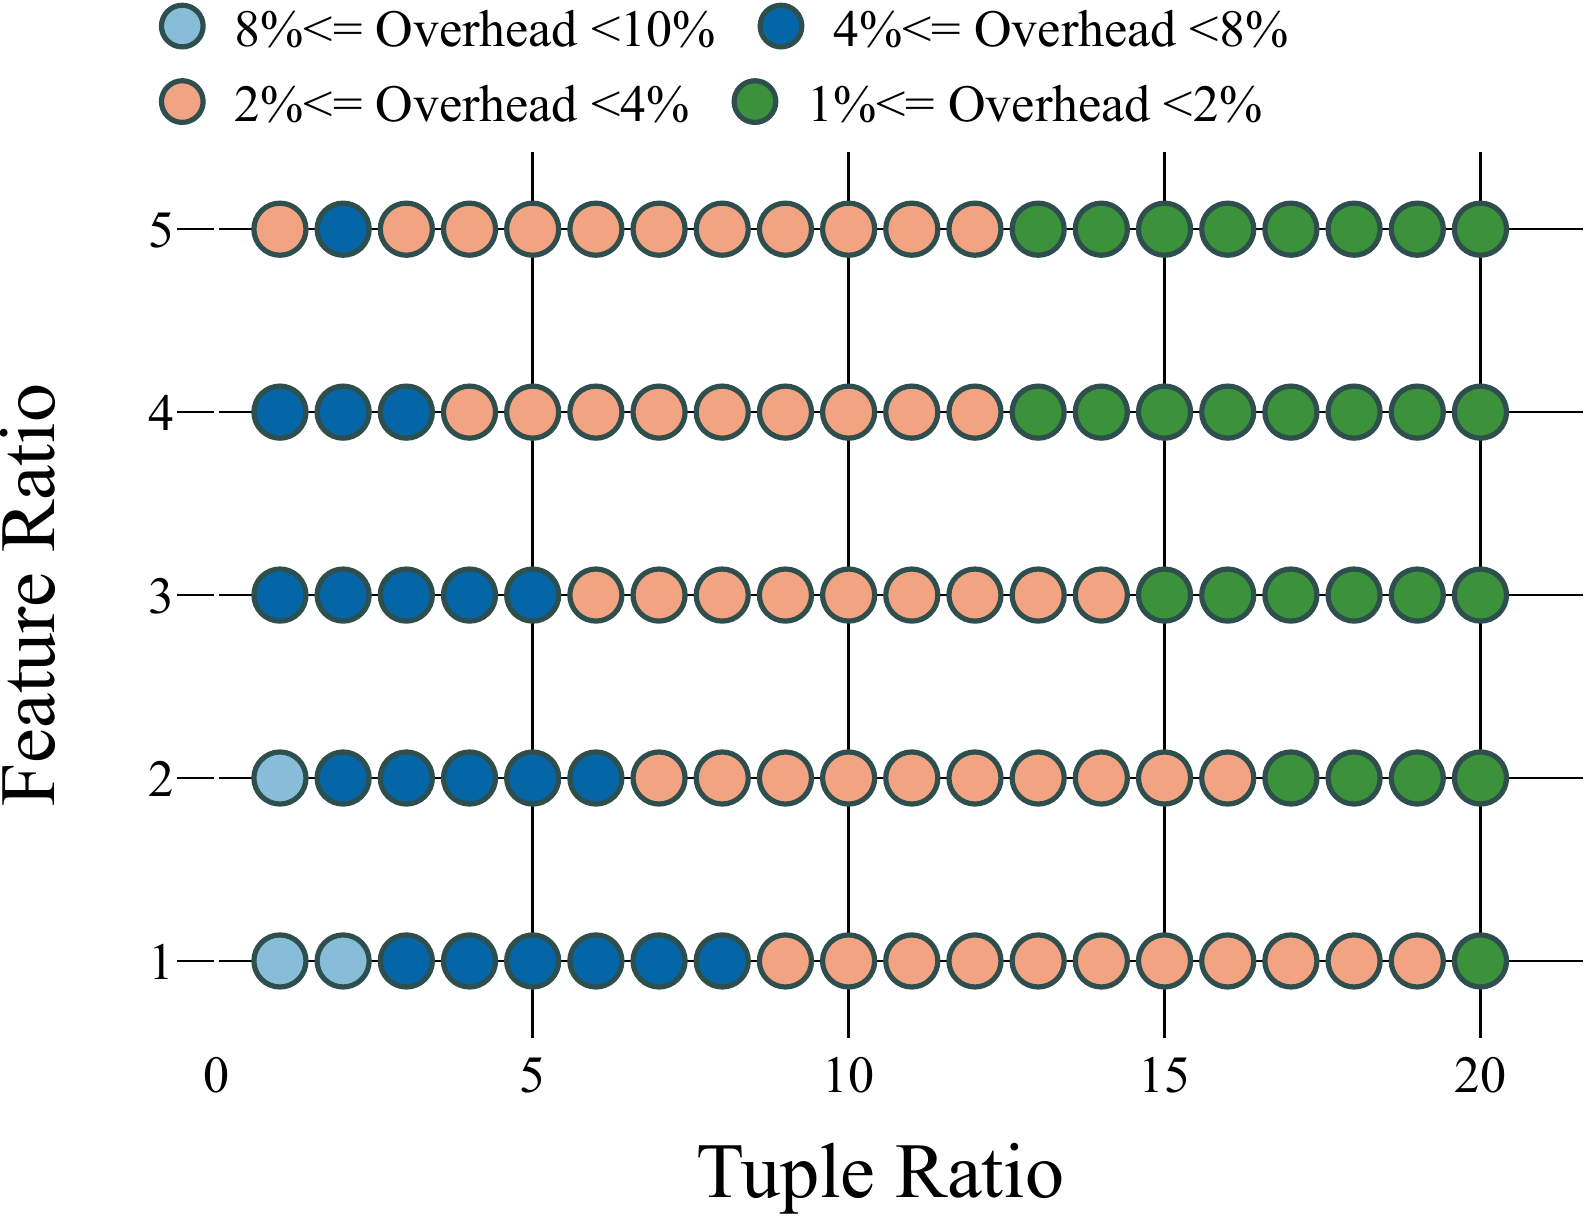}}
 \figspb\figspb\figspb
 \caption{$RW_{find}$ overhead as a percentage (\%) of the total time ($Q_{exec}+ RW_{fond}$) for pipelines 1.16 and 1.18}
 \figspc
 \label{fig:la-overhead-2}
\end{figure*}
